# Supplementary material for: Scaffold Embeddings: Learning the Structure Spanned by Chemical Fragments, Scaffolds and Compounds
Source: arXiv:2103.06867 source file (2021-03-11)
Supplement: Supplementary file 1 [file appendix.tex]

\documentclass[../main.tex]{subfiles}

\begin{document}
% \section*{SI}
% \textit{This needs to be moved to a separate document from the main text for submission. }
% \subsection{Constructing the dataset}
% We construct the dataset from the SAVI 2020 release, which contains over 1.3B enumeated smiles with information including predicted reactions. We utilize the positive set, which is reactions which indicate no extraneous problems. 

% From this dataset, we utilize RDKit to create a set with each compound and its general BM scaffold unsaturated hetero bonds on main framework.

% We create the extender model, $\hat{E}$ which takes a scaffold group and extends it. We call the dataset $E_\mathcal{D}$ which consists of scaffold groups translated to an instantiation of the group from SAVI dataset. Each dataset has the smiles randomized. 

% \subsection{Model training parameters}
% The ONMT toolkit was utilized for training. A vocabulary for smiles was created sampling 1M SMILES from the $E_\mathcal{D}$ dataset. Code preparation and model parameters were decided based on prior works, with a focus on \cite{schwaller2019molecular}. 

% \subsection{Example QSAR series}

\end{document}
